# Supplementary material for: Are you sure? Modelling Drivers' Confidence Judgments in Left-Turn Gap Acceptance Decisions
Source: arXiv:2403.06496 source file (2024-03-16)
Supplement: Supplementary file 1 [file Supplementary_information___Are_you_sure__Modelling_the_Confidence_of_a_Driver_in_Left_Turn_Gap_Acceptance_Decisions.pdf]

# Supplementary information for “Are you sure? Modelling the Confidence of a Driver in Left-Turn Gap Acceptance Decisions”

Floor Bontje[1], Arkady Zgonnikov [1,2]

This supplementary information document provides the following appendices: A) Figures of the linear mixed-effects models of decision behaviour, decision response time and confidence, B) an overview of the random effects terms present in the linear mixed effects models, C) linear mixed effects models describing the action dynamics velocity and distance to the centre of the intersection, D) correlations between the decision response time and the initial throttle operation moment, between confidence and decision response time and between confidence and the initial throttle operation moment, E) an explanation of the optimisation of the model parameters, and F) an explanation about the excluded left-turns.

## Appendix A - Figures, LME models

### Decision behaviour

$$Pr_{go} \sim distance + TTA + (1|ID)$$

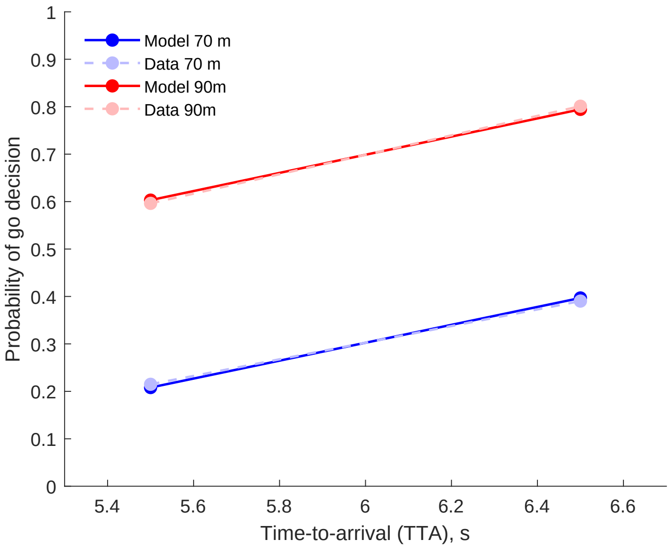


Fig. 1: Linear mixed effects model of the probability of making ”go” decisions

[1] *Department of Cognitive Robotics, Faculty of Mechanical, Maritime and MaterialsEngineering, Delft University of Technology, Netherlands*
[2] *AiTech, Delft University of Technology, Netherlands*

## Decision response time

$$RT \sim distance * decision + TTA * decision + (decision|ID)$$

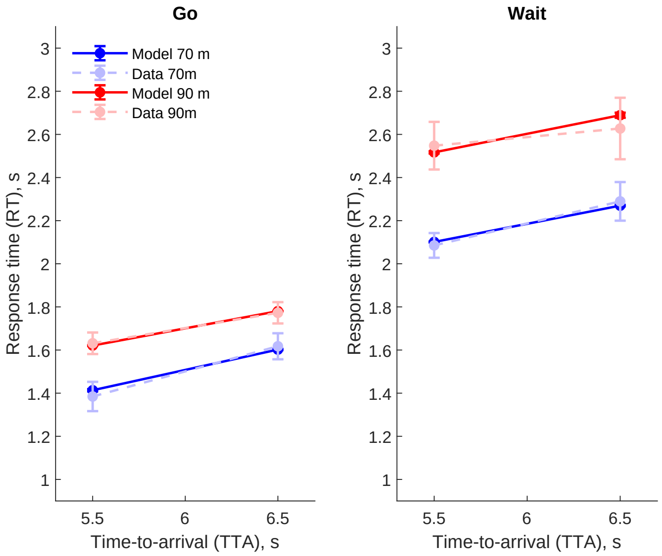


Fig. 2: Linear mixed effects model of the decision response time

## Confidence

$$Conf \sim RT * decision + distance * decision + TTA * decision + (decision|ID)$$

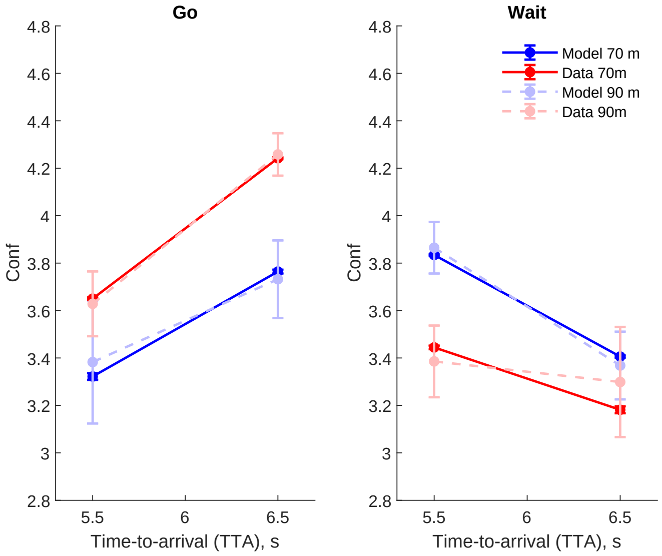


Fig. 3: Linear mixed effects model of confidence based on the decision response time, distance, time-to-arrival and decision

$$Conf \sim Thr_{int} * decision + distance * decision + TTA * decision + (decision|ID)$$

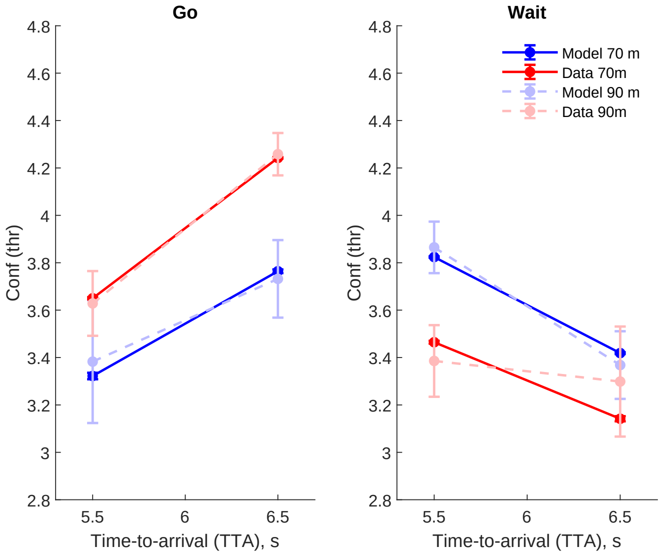


Fig. 4: Linear mixed effects model of confidence based on the initial throttle operation moment, distence, time-to-arrival and decision

## Appendix B - Random Effects

In order to account for the effects of individual differences between participants, all regression models have a random effects term (1| ID) or (decision | ID).

### Decision behaviour

We investigated the influence of the distance and time-to-arrival conditions by using the following linear mixed effect model: $Pr_{go} \sim distance + TTA + (1|ID)$ The random effects describing the influence of individual differences has a standard deviation 0.3978 of and 95% confidence interval of [0.3839, 0.4122]. For ten of the seventeen participants, an additional ($\alpha$ = 0.05) intercept was found (table 7).

| Estimate | pValue |
|---|---|
| 0.13796 | 0.034472 |
| -0.24048 | 0.00023872 |
| 0.13491 | 0.037971 |
| -0.21088 | 0.0013205 |
| 0.42177 | 1.2186e-10 |
| -0.26047 | 6.7498e-05 |
| -0.15967 | 0.01408 |
| 0.1417 | 0.033149 |
| -0.42763 | 1.1548e-09 |
| 0.34158 | 1.7393e-07 |

TABLE 1: Random effect coefficient of the intercept for the decision probability, capturing individual differences.

### Response time

The effect of the time-to-arrival and distance conditions was investigated with the following linear mixed effects model, $RT \sim distance * decision + TTA * decision + (decision|ID)$. The model accounts for individual differences with the random effects, consisting of a random intercept and a random decision slope (additional term for “wait” decision) (Table 8).

| | Std | 95% CI interval |
|---|---|---|
| Intercept | 0.25022 | 0.16431, 0.38105 |
| Wait decision | 0.34325 | 0.22103, 0.53306 |

TABLE 2: Random effects for the linear mixed effects model of the response time (RT), describing the influence of individual differences for different decision outcomes.

We found a random effect ($\alpha$ = 0.05) of the intercept for six participants (Table 9) and an additional random effect for the wait decision for seven participants (Table 10).

### Confidence (RT)

The effects of the response time, time-to-arrival and distance on confidence were investigated with the following linear mixed effects model: $Conf \sim RT * decision + TTA * decision + distance * decision + (decision|ID)$ The model accounts for individual differences with the random effects, consisting of a random intercept and a random decision slope (additional term for “wait” decision) (see table 11).

| Estimate | pValue |
|---|---|
| -0.32815 | 0.0051979 |
| 0.37553 | 0.0020354 |
| -0.27047 | 0.021912 |
| 0.74597 | 1.1226e-09 |
| -0.29145 | 0.012199 |
| 0.7309 | 0.0013217 |

TABLE 3: RT: Random effect coefficient of the intercept, capturing individual differences.

| Estimate | pValue |
|---|---|
| 0.51067 | 1.2307e-09 |
| -0.5062 | 1.2217e-07 |
| 0.20642 | 0.015385 |
| -0.23606 | 0.0018559 |
| -0.25012 | 0.0022344 |
| 0.18155 | 0.032157 |
| -0.25454 | 0.00091624 |

TABLE 4: RT: Random effect coefficient of the “wait” decision, describing individual differences

| | Std | 95% CI interval |
|---|---|---|
| Intercept | 0.51158 | 0.34788, 0.75232 |
| Wait decision | 0.48767 | 0.31956, 0.74422 |

TABLE 5: Random effects for the linear mixed effects model of confidence (response time), describing the influence of individual differences for different decision outcomes.

We found a random effect ($\alpha$ = 0.05) of the intercept for five participants (table 12) and an additional random effect for the wait decision for nine participants (table 13).

| Estimate | pValue |
|---|---|
| -0.42034 | 0.038575 |
| -0.56695 | 0.004159 |
| 0.63415 | 0.0014371 |
| 1.0984 | 6.1472e-08 |
| -0.61043 | 0.009719 |

TABLE 6: Confidence (RT): Random effect coefficient of the intercept, capturing individual differences.

| Estimate | pValue |
|---|---|
| 0.66059 | 0.00014618 |
| -0.49468 | 0.0026842 |
| -0.58171 | 0.00071363 |
| 0.35686 | 0.039236 |
| 0.97672 | 2.7953e-10 |
| -0.67047 | 5.7792e-05 |
| -0.51608 | 0.010064 |
| -0.6033 | 0.00097385 |
| 0.54496 | 0.0014252 |

TABLE 7: Confidence (RT): Random effect coefficient of the “wait” decision, describing individual differences

### Confidence (throttle)

The effects of the first moment in time of using the gas throttle after the appearances of the oncoming vehicle, time-to-arrival and distance on confidence were investigated with the following linear mixed effects model: $Conf \sim Thr_{int} * decision + TTA * decision + distance * decision + (decision|ID)$ The model accounts for individual differences with the random effects, consisting of a random intercept and a random decision slope (additional term for "wait" decision) (see table 14).

| | Std | 95% CI interval |
|---|---|---|
| Intercept | 0.45881 | 0.31474, 0.66882 |
| Wait decision | 0.49196 | 0.32783, 0.73825 |

TABLE 8: Random effects for the linear mixed effects model of confidence (throttle), describing the influence of individual differences for different decision outcome.

We found a random effect ($\alpha$ = 0.05) of the intercept for four participants (table 15) and an additional random effect for the wait decision for nine participants (table 16).

| Estimate | pValue |
|---|---|
| -0.6084 | 0.003291 |
| 0.75733 | 0.00024556 |
| 1.1477 | 3.4713e-08 |
| -0.62541 | 0.010011 |

TABLE 9: Confidence (CT): Random effect coefficient of the intercept, capturing individual differences.

| Estimate | pValue |
|---|---|
| 0.51859 | 0.0054811 |
| -0.57188 | 0.00063699 |
| 0.34505 | 0.039499 |
| 0.94403 | 4.177e-10 |
| -0.54311 | 0.00075716 |
| -0.58911 | 0.0027873 |
| -0.4385 | 0.013682 |
| -0.3781 | 0.016327 |
| 0.53283 | 0.001304 |

TABLE 10: Confidence (CT): Random effect coefficient of the "wait" decision, describing individual differences

## Appendix C - Action Dynamics, LME

The effect of confidence on the two measures of action dynamics, velocity profile and distance to centre of intersection, was investigated with the linear mixed effects models who is defined in general by: $Metric \sim Conf * decision + (1|ID)$.

For both measures four different metrics were taken into account: maximum/minimum value, deviation from the individual mean, deviation from the group mean and the RMSD.

### Velocity

#### Maximum velocity

| | Estimate | Std. Error | t-score | pValue |
|---|---|---|---|---|
| Intercept | 9.9337 | 0.44954 | 22.097 | 3.8434e-94 |
| Confidence | 0.097675 | 0.080369 | 1.2153 | 0.22442 |
| Decision wait | -0.26592 | 0.40842 | -0.65111 | 0.51508 |
| Decision wait: conf. | -0.13321 | 0.10769 | -1.237 | 0.21629 |

TABLE 11: Fixed coefficients of the linear mixed effects model describing the relation between confidence and the maximum value of the velocity profile.

| | Std | 95% CI interval |
|---|---|---|
| Intercept | 1.3148 | 0.92872, 1.8612 |

TABLE 12: Random effects of the linear mixed effects model describing the relation between confidence and the maximum value of the velocity profile.

#### Deviation from the individual mean

This model has a Hessian matrix with NaNs or Infs, which indicates that the model has more covariance parameters than supported by the data.

| | Estimate | Std. Error | t-score | pValue |
|---|---|---|---|---|
| Intercept | -0.18554 | 0.16697 | -1.1112 | 0.26666 |
| Confidence | 0.047861 | 0.04165 | 1.1491 | 0.25069 |
| Decision wait | 0.051122 | 0.22532 | 0.22689 | 0.82054 |
| Decision wait: conf. | -0.01007 | 0.058309 | -0.1727 | 0.86291 |

TABLE 13: Fixed coefficients of the linear mixed effects model describing the relation between confidence and the deviation from the individual mean of the distance to the velocity profile.

| | Std | 95% CI interval |
|---|---|---|
| Intercept | 2.6211e-16 NaN, NaN | |

TABLE 14: Random effects of the linear mixed effects model describing the relation between confidence and the deviation from the individual mean of the distance to the velocity profile.

#### Deviation from the group mean

| | Estimate | Std. Error | t-score | pValue |
|---|---|---|---|---|
| Intercept | -0.66223 | 0.29141 | -2.2725 | 0.023197 |
| Confidence | 0.10768 | 0.048922 | 2.2011 | 0.027879 |
| Decision wait | 0.75535 | 0.24851 | 3.0396 | 0.0024095 |
| Decision wait: conf. | -0.092263 | 0.065537 | -1.4078 | 0.15939 |

TABLE 15: Fixed coefficients of the linear mixed effects model describing the relation between confidence and the deviation from the group mean of the velocity profile.

| | Std | 95% CI interval |
|---|---|---|
| Intercept | 0.90075 | 0.63756, 1.2726 |

TABLE 16: Random effects of the linear mixed effects model describing the relation between confidence and the deviation from the group mean of the velocity profile.

#### RMSD

| | Estimate | Std. Error | t-score | pValue |
|---|---|---|---|---|
| Intercept | 0.98234 | 0.16598 | 5.9184 | 4.0042e-09 |
| Confidence | -0.060233 | 0.035916 | -1.6771 | 0.093731 |
| Decision wait | 0.5175 | 0.1831 | 2.8263 | 0.0047707 |
| Decision wait: conf. | 0.0314 | 0.048229 | 0.65106 | 0.51511 |

TABLE 17: Fixed coefficients of the linear mixed effects model describing the relation between confidence and the RMSD of the distance to the velocity profile.

| | Std | 95% CI interval |
|---|---|---|
| Intercept | Intercept | 0.35621 0.24773, 0.5122 |

TABLE 18: Random effects of the linear mixed effects model describing the relation between confidence and the RMSD of the distance to the velocity profile.

## Distance to the centre of the intersection

### Minimum distance

| | Estimate | Std. Error | t-score | pValue |
|---|---|---|---|---|
| Intercept | 2.6499 | 0.19741 | 13.423 | 6.388e-39 |
| Confidence | -0.16805 | 0.04266 | -3.9393 | 8.5385e-05 |
| Decision wait | -0.72751 | 0.21748 | -3.3452 | 0.00084219 |
| Decision wait: conf. | 0.19404 | 0.057285 | 3.3874 | 0.0007236 |

TABLE 19: Fixed coefficients of the linear mixed effects model describing the relation between confidence and the minimum value of the distance to the centre of the intersection.

| | Std | 95% CI interval |
|---|---|---|
| Intercept | 0.42517 | 0.29627, 0.61017 |

TABLE 20: Random effects of the linear mixed effects model describing the relation between confidence and the minimum value of the distance to the centre of the intersection.

### Deviation from the individual mean

This model has a Hessian matrix with NaNs or Infs, which indicates that the model has more covariance parameters than supported by the data.

| | Estimate | Std. Error | t-score | pValue |
|---|---|---|---|---|
| Intercept | 0.16542 | 0.15874 | 1.0421 | 0.29755 |
| Confidence | -0.042672 | 0.039598 | -1.0776 | 0.28137 |
| Decision wait | -0.26849 | 0.21422 | -1.2534 | 0.21027 |
| Decision wait: conf. | 0.071649 | 0.055437 | 1.2925 | 0.1964 |

TABLE 21: Fixed coefficients of the linear mixed effects model describing the relation between confidence and the deviation from the individual mean of the distance to the centre of the intersection.

| | Std | 95% CI interval |
|---|---|---|
| Intercept | 0 | NaN, NaN |

TABLE 22: Random effects of the linear mixed effects model describing the relation between confidence and the deviation from the individual mean of the distance to the centre of the intersection.

### Deviation from the group mean

| | Estimate | Std. Error | t-score | pValue |
|---|---|---|---|---|
| Intercept | 0.40604 | 0.22444 | 1.8091 | 0.070624 |
| Confidence | -0.10937 | 0.044829 | -2.4397 | 0.014813 |
| Decision wait | -0.64016 | 0.2281 | -2.8065 | 0.0050717 |
| Decision wait: conf. | 0.17602 | 0.06012 | 2.9279 | 0.0034634 |

TABLE 23: Fixed coefficients of the linear mixed effects model describing the relation between confidence and the deviation from the group mean of the distance to the centre of the intersection.

| | Std | 95% CI interval |
|---|---|---|
| Intercept | 0.57 | 0.40107, 0.81009 |

TABLE 24: Random effects of the linear mixed effects model describing the relation between confidence and the deviation from the group mean of the distance to the centre of the intersection.

### RMSD

| | Estimate | Std. Error | t-score | pValue |
|---|---|---|---|---|
| Intercept | 1.4447 | 0.12608 | 11.459 | 3.1844e-29 |
| Confidence | -0.074056 | 0.02703 | -2.7397 | 0.00622 |
| Decision wait | 0.058083 | 0.13776 | 0.42162 | 0.67336 |
| Decision wait: conf. | 0.043074 | 0.094796 | 1.187 | 0.23543 |

TABLE 25: Fixed coefficients of the linear mixed effects model describing the relation between confidence and the deviation from the group mean of the distance to the centre of the intersection.

| | Std | 95% CI interval |
|---|---|---|
| Intercept | 0.27727 | 0.19324, 0.39783 |

TABLE 26: Random effects of the linear mixed effects model describing the relation between confidence and the RMSD of the distance to the centre of the intersection.

## APPENDIX D - CORRELATIONS

In the research, several potential correlations were investigated:

1) Decision response time – Initial throttle operation moment
2) Confidence – Decision response time
3) Confidence – Initial throttle operation moment

### Decision response time - Initial throttle operation moment

| Decision | Correlation coefficient (r) | pValue |
|---|---|---|
| All | 0.2332 | 2.0647e-20 |
| Go | 0.2818 | 1.6121e-15 |
| Wait | -0.2409 | 1.4624e-11 |

TABLE 27: Correlation coefficients between decision response time (RT) and the initial throttle operation moment.

### Confidence - Decision response time

| Decision | Correlation coefficient (r) | pValue |
|---|---|---|
| All | -0.2729 | 1.2874e-27 |
| Go | -0.2114 | 3.1298e-09 |
| Wait | -0.2490 | 2.8442e-12 |

TABLE 28: Correlation coefficients between confidence and the decision response time (RT).

| TTA\distance | 70 m | 90 m |
|---|---|---|
| 5.5 seconds | -0.49 (p=4.13e-06) | -0.34 (p=2.5e-07) |
| 6.5 seconds | -0.22 (p=0.0062) | -0.35 (p=2.5e-10) |

TABLE 29: Correlation coefficients between RT and confidence judgements – in each traffic condition for ”Go” decisions.

| TTA\distance | 70 m | 90 m |
|---|---|---|
| 5.5 seconds | -0.23 (p=6.4e-05) | -0.24 (p=0.0028) |
| 6.5 seconds | -0.19 (p=0.0038) | -0.13 (p=0.27) |

TABLE 30: Correlation coefficients between RT and confidence judgements – in each traffic condition for ”wait” decisions.

### Confidence - Initial throttle operation moment

| Decision | Correlation coefficient (r) | pValue |
|---|---|---|
| All | -0.2224 | 1.1645e-18 |
| Go | -0.2735 | 1.1195e-14 |
| Wait | -0.1591 | 9.8448e-06 |

TABLE 31: Correlation coefficients between confidence and the initial throttle operation moment.

| TTA\distance | 70 m | 90 m |
|---|---|---|
| 5.5 seconds | -0.44 (p=3.3e-05) | -0.46 (p=4.0e-13) |
| 6.5 seconds | -0.37 (p=2.5e-06) | -0.27 (p=1.5e-06) |

TABLE 32: Correlation coefficients between initial throttle operation moment and confidence judgements – in each traffic condition for ”Go” decisions.

| TTA\distance | 70 m | 90 m |
|---|---|---|
| 5.5 seconds | -0.055 (p=0.35) | -0.089 (p=0.28) |
| 6.5 seconds | -0.21 (p=0.0014) | -0.32 (p=0.0040) |

TABLE 33: Correlation coefficients between initial throttle operation moment and confidence judgements – in each traffic condition for ”wait” decisions.

## Appendix E - Optimisation of Model Parameters

For optimisation of the model parameters, we made use of the "fmincon" function of MATLAB R2020a. The function searches for the set of parameters which result in a (local) minimum of the loss function of the performance of the model.

### Lossfunctions

For the loss functions of the performance of the models, we made use of the weight least squares (WLS) and the root mean square error (RMSE) for respectively the decision and confidence models.

#### *Decision models*

To train the decision models, we made use of a newly defined loss function build up from the WLS of the model prediction. The WLS was calculated with the use of vincentized distributions [?]. For each of the four different conditions present in the experiment, the WLS was calculated, using two separate terms describing the WLS for "go" and "wait" decisions. The total sum of the WLS over all conditions was used as loss function.

#### *Confidence models*

For the confidence models, the root mean square error (RMSE) was used as loss function, which can be described by the following equations:

$$RMSE = \sqrt{\frac{\sum(Conf_{pr} - Conf_{expr})^2}{N_conf}}$$

$$Conf_i = [\mu_{conf,go,i}, \mu_{conf_wait,i}]$$

$\mu_{conf,decision,i}$ contains the mean confidence values for the four conditions in the specified decision of the prediction or the experiment. $N_{conf}$ is the number of measuring points, so $N_{conf} = 4 * 2 = 8$.

### Parameters

The "fmincon" function starts searching for an optimal set of parameters round an initial set of parameters, which must be defined in advance.

#### *Decision model*

The initial set of parameters used to train the decision models was obtained with the use of the optimisation code "03_fit_model.py" which accompanied our baseline decision model [?]. This optimisation was focused on the prediction of left-turn gap acceptance decision behaviour by a dynamic drift diffusion model only accounting for "go"-decisions. This set of initial parameters was as a result not able to predict wait decisions accurately.

The newly defined loss function was used in combination with the found initial parameters to find the parameter set describing both "go" and "wait" decisions for a dynamic drift-diffusion model and for a race model.

| | WLS | $\alpha$ | beta | $b_0$ | k | $\mu_n d$ | $\sigma_n d$ | $\theta_{crit}$ |
|---|---|---|---|---|---|---|---|---|
| Initial | 3.08 | 0.985 | 0.101 | 1.14 | 0.357 | 1.40 | 0.117 | 13.7 |
| DDM | 1.53 | 1.12 | 0.109 | 1.41 | 0.396 | 1.51 | 0.140 | 14.0 |

TABLE 34: Initial trained model ("go") and DDM models ("go" and "wait"): a) comparison of performance of the decision models, mean WLS over 10 models, b) parameter values found through optimisation.

For the race model, the drift-rate parameter ($\alpha$) is assumed to be decision dependent. Besides, we investigated the effect on the performance of the model by decision dependent initial boundaries ($b_0$) and critical values of the generalised gap ($\theta_{crit}$). The present non-decision time, the sensitivity of the boundary and the definition of the generalised gap were defined as being decision independent, i.e., similar for both evidence accumulators. In order to test the optimisation method used, we also investigated the effect on the performance of the model by defining all model parameters decision dependent. If all model parameters are decision dependent, this should result in the best performance (lowest WLS).

The results of the parameter optimisation showed that the race model with decision dependent drift-rate parameters and the race model with both decision dependent drift-rate parameters as well as critical values of the generalised gap resulted the highest improvement of the performance (lowest WLS-values). These results are based on the initial parameter set of the drift-diffusion model which was not able to predict both "go" and "wait" decisions. Therefore, we additionally investigated whether the use of the optimal parameters for the drift-diffusion model could improve the optimisation of the race model with decision dependent drift-rate parameters and the race model with both decision dependent drift-rate parameters as well as decision dependent critical values of the generalised gap. Thereby, we found that the race model is able to describe the decision behaviour with the decision dependent drift-rate parameter and the critical generalised gap value trained with the use of the drift-diffusion model parameters describing "go" and "wait" decisions (table 41 and table 42, Figure 15).

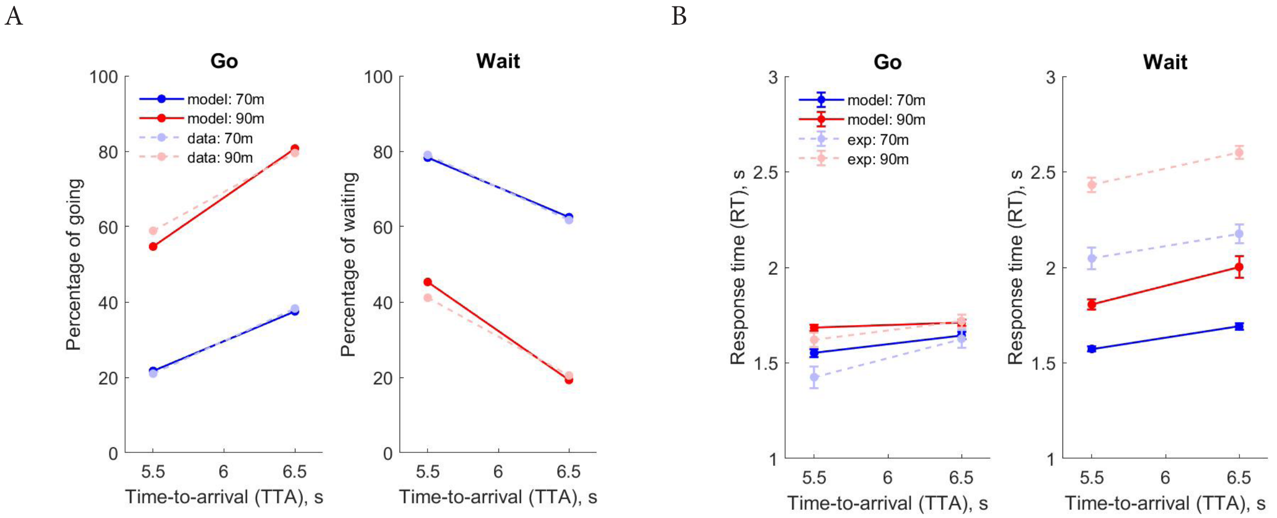


Fig. 5: Performance of drift-diffusion decision model, trained for "go" decisions (initial parameters).

| | WLS | $\alpha$ | $\beta$ | $b_0$ | k | $\mu_{ND}$ | $\sigma_{ND}$ | $\theta_{crit}$ |
|---|---|---|---|---|---|---|---|---|
| race ($\alpha$) | 1.67 | Go: 0.838<br>Wait: 0.901 | 0.117 | 1.49 | 0.38 | 1.50 | 0.326 | 14.2 |
| race ($\alpha$&$b_0$) | 2.62 | Go: 1.52<br>Wait:1.32 | 0.0938 | Go: 0.504<br>Wait:0.500 | 0.101 | 1.85 | 0.207 | 13.3 |
| race ($\alpha$&$\theta_{crit}$) | 1.73 | Go: 1.03<br>Wait: 1.13 | 0.112 | 1.21 | 0.341 | 1.51 | 0.123 | Go: 13.8<br>Wait: 13.7 |
| race (all) | 0.48 | Go: 0.810<br>Wait:1.47 | Go:0.0988<br>Wait:0.102 | Go:0.966<br>Wait:1.17 | Go:0.394<br>Wait:0.390 | Go:1.35<br>Wait:1.84 | Go:0.131<br>Wait:0.124 | Go:13.8<br>Wait:13.8 |

TABLE 35: Race model mean performance (WLS) over 10 models, trained with initial parameters. Influence of different decision dependent parameters.

| | WLS | $\alpha$ | $\beta$ | k | $b_0$ | $\mu_{ND}$ | $\sigma_{ND}$ | $\theta_{crit}$ |
|---|---|---|---|---|---|---|---|---|
| race ($\alpha$) | 1.73 | Go: 1.05<br>Wait: 1.24 | 0.105 | 1.24 | 0.413 | 1.53 | 0.129 | 13.7 |
| race ($\alpha$ & $\theta_{crit}$) | 1.33 | Go: 1.06<br>Wait: 1.05 | 0.108 | 1.21 | 0.454 | 1.54 | 0.128 | Go: 14.0<br>Wait: 13.5 |

TABLE 36: Race model mean performance (WLS) over 10 models, trained with parameters of the drift-diffusion model. Influence of different decision dependent parameters.

### *Confidence models*

The confidence models presented in this paper were built on the decision model by adding four additional free parameters, describing sensitivity and bias for both decisions, and by potentially allowing for additional evidence accumulation.

**Sensitivity and bias parameters**

The initial values of the additional confidence model parameters describing sensitivity and the bias were found using a linear regression model of the relation between confidence and the input value ($V_c$). However, the sensitivity parameters can only be positive and linear regression models cannot be constrained. As a result, we trained the confidence models with the use of the "fmincon" function, thereby including the constraint that the sensitivity parameters should be positive.

**Inter-judgement times**

Two of the four confidence models accounted for additional evidence accumulation after the decision was made. The time evidence continues to accumulate, inter-judgement time ($\tau$), could not be measured during the experiment and thus had to be modelled. In order to do so, the effect of the different values of the inter-judgement time on the RMSE was calculated manually, over a time scale from zero to 2.5 seconds with a time interval of 0.01 seconds (Figure 7). The RMSE of the confidence models with a specific inter-judgment time, used in the comparison of the effect of different inter-judgement times, was defined as the mean RMSE over 5 models. The model parameters of the confidence model were fitted separately for each investigated inter-judgment time with the use of a linear regression model, where all sensitivity parameters smaller or equal to zero were defined as zero due to the constraint that the sensitivity parameters must be positive.

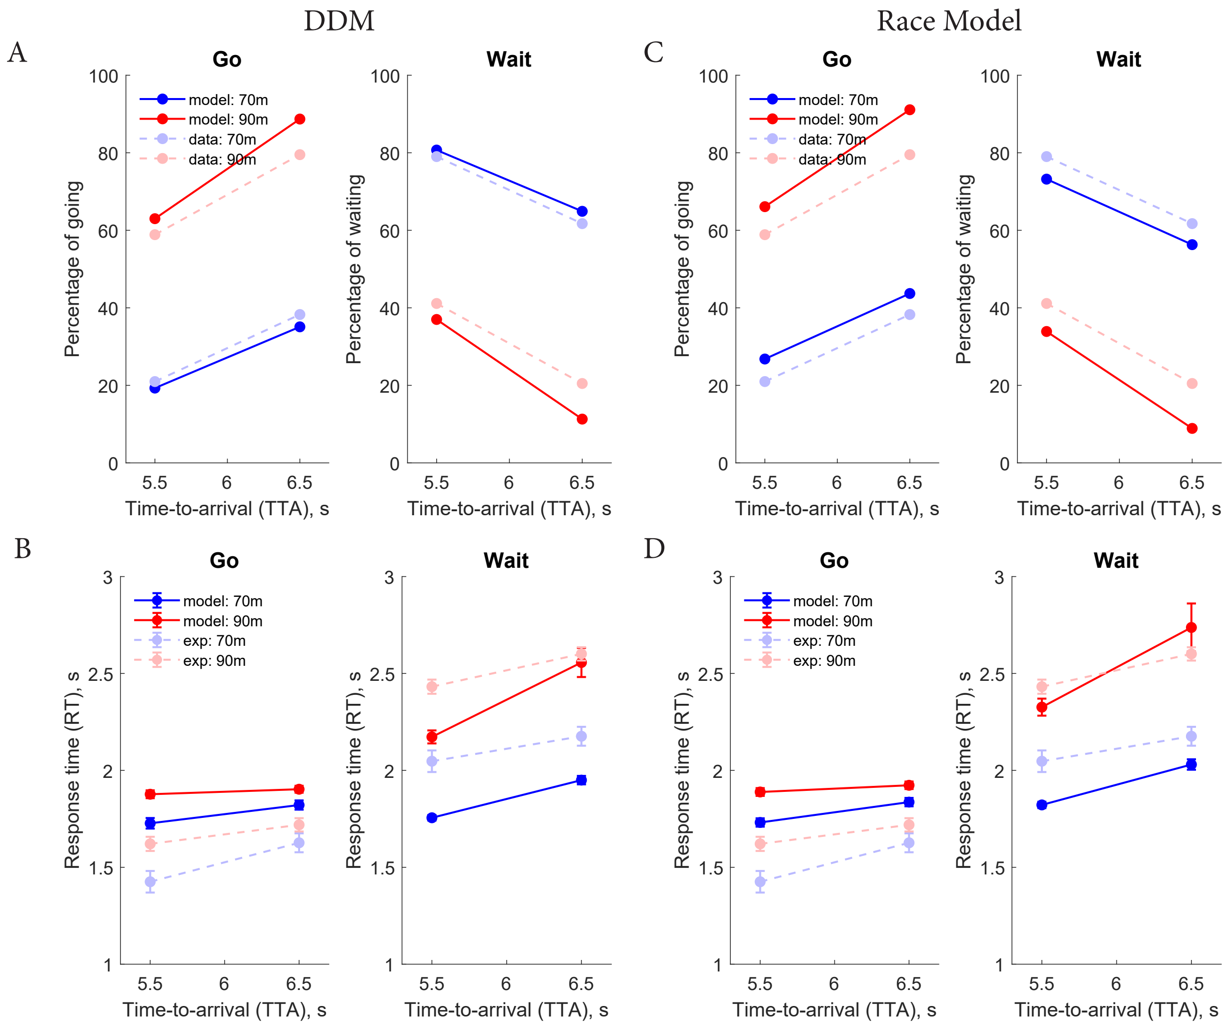


Fig. 6: Performance of drift-diffusion model (DDM) and race model with trained parameters.

The results show that the performance of the models is affected by the inter-judgement time until the inter-judgement time reaches a value of approximately 1.2 seconds after which the performance remains constant (Figure 7). At the inter-judgement time of 1.2 seconds, both models perform optimal. This finding suggests that the model is over parameterised or fails to correctly describe the evidence accumulation process for a longer period of time after the decision is made. The model does for example not account for the moment in time in which the decision is made or in which the oncoming vehicle has passed.

## Model parameters

An overview of the finial confidence model parameters used in the confidence models presented in the paper.

| | Bias parameter | Sensitivity parameter |
|---|---|---|
| Model 1: DDM, $\tau = 0s$ | Go: 1.17<br>Wait: 3.10 | Go: 3.42<br>Wait: 0.707 |
| Model 2: DDM, $\tau = 1.2s$ | Go: 4.05<br>Wait: 2.03 | Go: 0.23<br>Wait: 0.410 |
| Model 3: Race model, $\tau = 0s$ | Go: 0.876<br>Wait: 3.74 | Go: 3.74<br>Wait: 0.552 |
| Model 4: Race model, $\tau = 1.2s$ | Go: 3.87<br>Wait: 1.63 | Go: 0.22<br>Wait: 0.44 |

TABLE 37: Confidence model parameters, used for the different presented confidence models.

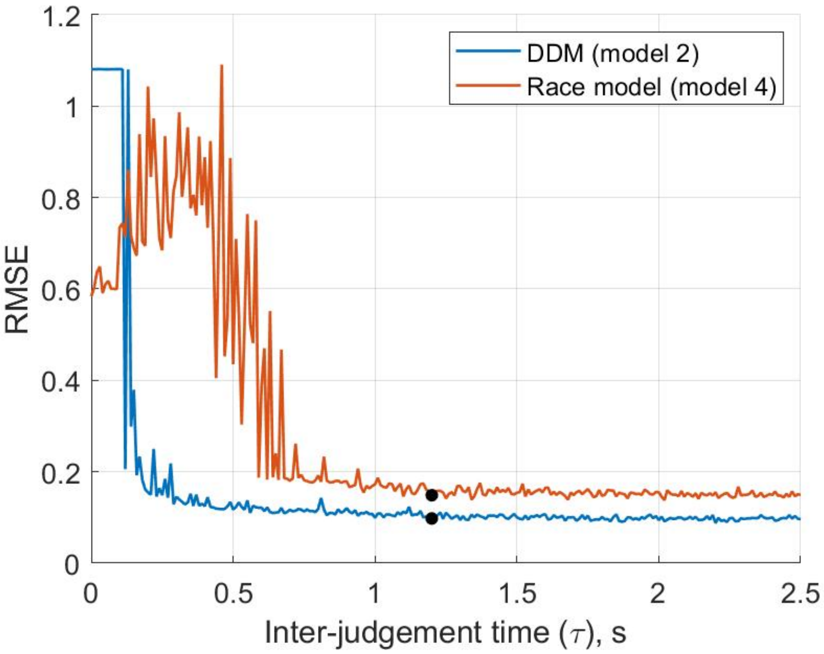


Fig. 7: Effect of different inter-judgement times on the performance (RMSE) of the confidence model based on the drift-diffusion decision model (model 2) and the confidence model based on the race model (model 4). The black point indicates the inter-judgement time used for the final confidence models (1.2 seconds)

## Appendix F - Excluded Left-turns

The data analysis in this study was restricted to the left-turn trials in which the indicated decision was actually conducted. We excluded all changes of mind, situations in which the participant carried out a different decision than indicated, as well as the trials in which the participants did not indicate their decision (by failing to press the designated button).

In 3.4 % of all the left-turn decisions, changes of mind were present, of which in 83.9% of the cases the participant indicated a “go” decision and performed a “wait” decision. In 2.2% of all left-turn decisions, no button presses were present. In 83.33% of the cases in which participates failed to press the button, they performed a “go” decision.
